# Supplementary material for: Reinforcement Learning under Partial Observability Guided by Learned Environment Models
Source: arXiv:2206.11708 source file (2022-06-23)
Supplement: Supplementary file 1 [file appendix.tex]

\section{Appendix -- Learned Models}
In this appendix, we show two learned models for the \emph{first grid} example, 
one MDP model and one SMM model to illustrate their differences. Even though
they have only $19$ and $35$ states, respectively, they are hard to visualize. 
Therefore, we show only the initial part of both models in Fig.~\ref{fig:learned_model_zoom}. 
It can be seen that there are several self loop transitions in the initial SMM state. 
They produce the \emph{Wall} output, for instance, signalling that the agent navigating in the
gridworld cannot move \emph{West}, but bumps into a wall when trying to move west. 
Modeling the same functionality in the MDP requires 
two states, where one is labeled \emph{Wall}. These two states are the topmost states in the left part
of Fig.~\ref{fig:learned_model_zoom}. As another example, we can take a look at the transition labeled with 
the input \emph{East} and the output \emph{concrete} from the initial SMM state to the state \emph{s1}.
The transition models that by moving East, the agent moves onto concrete. The same transition appears
twice in the MDP model; once from the initial state and once from the state that is below and left of the 
initial state. This explains that more samples are required to learn MDP transitions and their probabilities.
In this particular case, the probabilities are actually simple to learn, as they equal to one, 
but in lower parts of the figure there are other probability values.

The complete models are shown in Fig.~\ref{fig:learned_first_grid_mdp} and 
Fig.~\ref{fig:learned_first_grid_smm}, respectively. It is apparent that the SMM model is 
considerably smaller and because of that also easier to analyze manually. 

\begin{figure}[h]
\begin{center}
 \includegraphics[width=.48\textwidth,trim=700 3100 2800 50,clip]{figures/learned_first_grid_mdp}
 \includegraphics[width=.48\textwidth,trim=1550 1300 1200 50,clip]{figures/learned_first_grid_smm}
\end{center}
 \caption{Initial part of the learned MDP model of the first gridworld example (left) and the corresponding 
 initial part of the learned SMM model (right).}
 \label{fig:learned_model_zoom}
 \end{figure}
\begin{figure}
\begin{center}
 \includegraphics[width=.85\textwidth]{figures/learned_first_grid_mdp}
\end{center}
 \caption{Learned MDP model of the first gridworld example.}
 \label{fig:learned_first_grid_mdp}
 \end{figure}
\begin{figure}
\begin{center}
 \includegraphics[width=.85\textwidth]{figures/learned_first_grid_smm}
\end{center}
 \caption{Learned SMM model of the first gridworld example.}
 \label{fig:learned_first_grid_smm}
\end{figure}

% \begin{figure}
% \begin{center}
%  \includegraphics[scale=0.25,trim=1550 1300 1200 50,clip]{figures/learned_first_grid_smm}
% \end{center}
%  \caption{Learned SMM model of the first grid world example (zoomed in).}
%  \label{fig:learned_first_grid_smm}
% \end{figure}

% trim=left bottom right top, clip
